# Supplementary material for: Pressure-induced structural dimerization in the hyperhoneycomb iridate $\beta$-Li$_2$IrO$_3$ at low temperatures
Source: arXiv:1905.08211 ancillary file (2019-05-30)
Supplement: Supplementary file 1 [file Li213_PRB_SUPPLEMENTAL.pdf]

# Pressure-induced structural dimerization in the hyperhoneycomb iridate β-$Li_2IrO_3$ at low temperatures

L.S.I. Veiga,[1,*] K. Glazyrin,[2] G. Fabbris,[3] C.D. Dashwood,[1] J.G. Vale,[1] H. Park,[4,5] M. Etter,[2] T. Irifune,[6,7] S. Pascarelli,[8] D.F. McMorrow,[1] T. Takayama,[9,10] H. Takagi,[9,10] and D. Haskel[3,†]

[1] *London Centre for Nanotechnology and Department of Physics and Astronomy, University College London, Gower Street, London WC1E6BT, UK*

[2] *Deutsches Elektronen-Synchrotron (DESY), Hamburg 22607, Germany*

[3] *Advanced Photon Source, Argonne National Laboratory, Argonne, Illinois 60439, USA*

[4] *Physics Department, University of Illinois at Chicago, Chicago, IL 60607*

[5] *Materials Science Division, Argonne National Laboratory, Lemont, Illinois, 60439, USA*

[6] *Geodynamics Research Center, Ehime University, Matsuyama, 790-8577, Japan*

[7] *Earth-Life Science Institute, Tokyo Institute of Technology, Tokyo, Japan*

[8] *European Synchrotron Radiation Facility, 71 Avenue des Martyrs, 38043 Grenoble, France*

[9] *Max Planck Institute for Solid State Research, Heisenbergstrasse 1, 70569 Stuttgart, Germany*

[10] *Department of Physics and Department of Advanced Materials, University of Tokyo, 7-3-1 Hongo, Tokyo, 113-0033, Japan*

(Dated: May 30, 2019)

## I. SUPPORTING DATA

Tables S1, S2, S5 and S6 summarizes the lattice parameters and atomic positions as a function of pressure for each identified crystal structure at $T = 50$ K. The R factor of the structural solutions is reported in Tables S3 ($Fddd$) and S4 ($C2/c$) along with the isotropic displacement parameter ($U_{iso}$), reciprocal space coverage, number of refined reflections, number of refined parameters and data completeness. The R factor is related to refinements on the square structure parameter $F^2$. For the $C2/c$ structures, the Li positions were fixed to the center of the $LiO_6$ octahedra. All Li and O sites have the same isotropic displacement parameters and $U_{iso}(Li) = U_{iso}(O)$ for the $C2/c$ structures. All the atomic positions were standardized using the software VESTA[1].

TABLE S1. Lattice parameters and atomic coordinates of $\beta$-$Li_2IrO_3$ with $Fddd$ (No. 70, $Z = 16$) space-group symmetry extracted from single crystal analysis at $T = 50$ K. $x = y = 1/8$ and $y = z = 1/8$ for the $16g$ and $16e$ Wyckoff positions, respectively.

| | P (GPa) | 0.2(1) | 0.5(1) | 2.5(1) | 3.2(1) | 3.5(1) | 4.2(1) |
|---|---|---|---|---|---|---|---|
| a | | 5.8664(10) | 5.8589(4) | 5.8585(5) | 5.8471(4) | 5.8415(6) | 5.821(2) |
| b | (Å) | 8.3836(4) | 8.3757(16) | 8.4734(2) | 8.4538(2) | 8.4501(3) | 8.4470(9) |
| c | | 17.6792(16) | 17.6740(7) | 16.8814(8) | 16.8424(8) | 16.8264(11) | 16.798(4) |
| Volume | (Å$^3$) | 869.48(17) | 867.31(18) | 838.02(8) | 832.52(7) | 830.57(11) | 825.9(4) |
| Ir (16$g$) | $z$ | 0.04151(5) | 0.04154(5) | 0.04654(2) | 0.04659(3) | 0.04665(2) | 0.04671(4) |
| Li1 (16$g$) | $z$ | 0.545(2) | 0.541(4) | 0.5426(12) | 0.5434(16) | 0.5435(14) | 0.543(2) |
| Li2 (16$g$) | $z$ | 0.381(4) | 0.382(3) | 0.3801(13) | 0.3786(18) | 0.3792(16) | 0.376(3) |
| O1 (16$e$) | $x$ | 0.355(3) | 0.361(4) | 0.3798(16) | 0.385(2) | 0.3798(19) | 0.370(3) |
| O2 (32$h$) | $x$ | 0.130(3) | 0.132(3) | 0.1410(10) | 0.1360(15) | 0.1396(11) | 0.144(2) |
| | $y$ | 0.3645(7) | 0.3645(7) | 0.3648(6) | 0.3652(9) | 0.3655(7) | 0.3663(10) |
| | $z$ | 0.0377(3) | 0.0383(3) | 0.0382(3) | 0.0387(5) | 0.0384(4) | 0.0389(6) |

TABLE S2. Lattice parameters and atomic coordinates of $\beta$-$Li_2IrO_3$ with $C2/c$ (No. 15, $Z = 8$) space-group symmetry extracted from single crystal analysis at $T = 50$ K.

| | P (GPa) | 2.5(1) | 3.2(1) | 3.5(1) | 4.2(1) | 6.5(1) | 8.2(1) | 9.4(1) |
|---|---|---|---|---|---|---|---|---|
| a | | 5.8487(11) | 5.852(5) | 5.843(2) | 5.830(3) | 5.776(2) | 5.748(2) | 5.732(3) |
| b | (Å) | 8.1071(4) | 8.0751(18) | 8.0610(7) | 8.0590(10) | 8.0297(6) | 7.9858(8) | 7.9628(9) |
| c | | 9.1979(19) | 9.190(7) | 9.167(4) | 9.167(5) | 9.115(4) | 9.096(5) | 9.074(5) |
| $\beta$ | ° | 107.04(2) | 107.24(1) | 107.05(5) | 107.03(6) | 106.74(5) | 106.80(6) | 106.82(6) |
| Volume | (Å$^3$) | 416.98(12) | 414.8(5) | 412.8(3) | 411.8(3) | 404.8(2) | 399.7(3) | 396.5(3) |
| Ir | $x$ | 0.07805(16) | 0.0771(2) | 0.07750(16) | 0.07714(14) | 0.0771(2) | 0.07693(19) | 0.07683(14) |
| | $y$ | 0.11562(6) | 0.11483(9) | 0.11451(7) | 0.11440(7) | 0.11403(8) | 0.11395(9) | 0.11373(7) |
| | $z$ | 0.42186(9) | 0.42246(13) | 0.42235(10) | 0.42257(9) | 0.42261(11) | 0.42261(11) | 0.42274(9) |
| Li1 | $x$ | 0.2500(15) | 0.250(2) | 0.2500(15) | 0.2500(13) | 0.2500(18) | 0.250(2) | 0.2500(15) |
| | $y$ | 0.3701(4) | 0.3676(7) | 0.3701(5) | 0.3703(4) | 0.3708(6) | 0.3705(8) | 0.3701(5) |
| | $z$ | 0.2500(9) | 0.2500(12) | 0.2500(9) | 0.2500(8) | 0.2500(10) | 0.2500(13) | 0.2500(9) |
| Li2 | $x$ | 0.4167(15) | 0.417(2) | 0.4167(15) | 0.4167(13) | 0.4167(18) | 0.417(2) | 0.4167(15) |
| | $y$ | 0.1217(4) | 0.1211(7) | 0.1215(5) | 0.1211(4) | 0.1211(6) | 0.1196(8) | 0.1212(5) |
| | $z$ | 0.0833(9) | 0.0833(12) | 0.0833(9) | 0.0833(8) | 0.0833(10) | 0.0833(13) | 0.0833(9) |
| O1 | $x$ | 0.231(4) | 0.235(5) | 0.242(4) | 0.234(3) | 0.234(5) | 0.221(5) | 0.230 (4) |
| | $y$ | 0.1150(10) | 0.1133(15) | 0.1145(11) | 0.1134(10) | 0.1134(13) | 0.1089(18) | 0.1137(12) |
| | $z$ | 0.251(2) | 0.247(3) | 0.246(2) | 0.250(2) | 0.252(3) | 0.262(3) | 0.256(3) |
| O2 | $x$ | 0.090(3) | 0.096(4) | 0.092(3) | 0.092(3) | 0.096(4) | 0.101(5) | 0.096(3) |
| | $y$ | 0.3604(13) | 0.353(2) | 0.3604(15) | 0.3609(12) | 0.3625(18) | 0.362(3) | 0.3603(16) |
| | $z$ | 0.4232(18) | 0.419(2) | 0.4231(19) | 0.4225(19) | 0.420(2) | 0.418(3) | 0.4185(19) |
| O3 | $x$ | 0.409(3) | 0.393(5) | 0.403(4) | 0.407(3) | 0.410(4) | 0.414(5) | 0.414(3) |
| | $y$ | 0.3711(12) | 0.3731(18) | 0.3679(14) | 0.3668(12) | 0.3650(18) | 0.363(3) | 0.3698(16) |
| | $z$ | 0.087(2) | 0.093(3) | 0.088(2) | 0.087(2) | 0.083(2) | 0.077(3) | 0.081(2) |

TABLE S3. R factors in %, reciprocal space coverage, number of refined reflections, number of refined parameters, the isotropic displacement parameter ($U_{\mathrm{iso}}$) and data completeness (in %) from the single crystal structural solution within the $Fddd$ space group. The R factors and $\chi^2$ values refer to the solution performed with the intensity threshold $I > 3\sigma(I)$. $U_{\mathrm{iso}}$ is given in Å$^2$ units.

| P (GPa) | 0.2(1) | 0.5(1) | 2.5(1) | 3.2(1) | 3.5(1) | 4.2(1) |
|---|---|---|---|---|---|---|
| R factor | 2.32 | 2.93 | 2.89 | 4.16 | 3.51 | 4.23 |
| Reciprocal space coverage | $-7 \leq H \leq 8$ | $-8 \leq H \leq 7$ | $-7 \leq H \leq 9$ | $-7 \leq H \leq 9$ | $-7 \leq H \leq 9$ | $-9 \leq H \leq 5$ |
| | $-17 \leq K \leq 17$ | $-17 \leq K \leq 17$ | $-17 \leq K \leq 17$ | $-17 \leq K \leq 17$ | $-17 \leq K \leq 17$ | $-17 \leq K \leq 15$ |
| | $-29 \leq L \leq 31$ | $-31 \leq L \leq 29$ | $-29 \leq L \leq 26$ | $-25 \leq L \leq 29$ | $-28 \leq L \leq 25$ | $-27 \leq L \leq 26$ |
| No. of ref. reflec. | 223 | 221 | 259 | 241 | 250 | 236 |
| No. of ref. param. | 13 | 13 | 10 | 10 | 10 | 13 |
| Data completeness | 32.5 | 31.5 | 31.5 | 31.1 | 29.9 | 32.4 |
| $U_{iso}$(Ir) | 0.00029(12) | 0.00311(14) | 0.00416(14) | 0.0063(2) | 0.00557(17) | 0.0048(2) |
| $U_{iso}$(Li1) | 0.002(4) | 0.007(5) | 0.0049(8) | 0.0056(12) | 0.0061(10) | 0.010(7) |
| $U_{iso}$(Li2) | 0.015(8) | 0.004(6) | 0.0049(8) | 0.0056(12) | 0.0061(10) | 0.013(8) |
| $U_{iso}$(O1) | 0.0009(12) | 0.0038(14) | 0.0049(8) | 0.0056(12) | 0.0061(10) | 0.007(2) |
| $U_{iso}$(O2) | 0.0023(9) | 0.0021(10) | 0.0049(8) | 0.0056(12) | 0.0061(10) | 0.0031(14) |

TABLE S4. R factors in %, reciprocal space coverage, number of refined reflections, number of refined parameters, the isotropic displacement parameter ($U_{\mathrm{iso}}$) and data completeness (in %) from the single crystal structural solution within the $C2/c$ space group. The R factors and $\chi^2$ values refer to the solution performed with the intensity threshold $I > 3\sigma(I)$. $U_{\mathrm{iso}}$ is given in Å$^2$ units.

| P (GPa) | 2.5(1) | 3.2(1) | 3.5(1) | 4.2(1) | 6.5(1) | 8.2(1) | 9.4(1) |
|---|---|---|---|---|---|---|---|
| R factor | 5.54 | 6.93 | 5.25 | 4.41 | 6.02 | 6.91 | 5.85 |
| Reciprocal space coverage | $-9 \leq H \leq 7$ | $-9 \leq H \leq 7$ | $-9 \leq H \leq 7$ | $-7 \leq H \leq 9$ | $-9 \leq H \leq 7$ | $-9 \leq H \leq 7$ | $-9 \leq H \leq 7$ |
| | $-16 \leq K \leq 16$ | $-16 \leq K \leq 16$ | $-16 \leq K \leq 16$ | $-16 \leq K \leq 16$ | $-16 \leq K \leq 16$ | $-16 \leq K \leq 16$ | $-16 \leq K \leq 16$ |
| | $-10 \leq L \leq 12$ | $-10 \leq L \leq 12$ | $-10 \leq L \leq 12$ | $-12 \leq L \leq 10$ | $-10 \leq L \leq 12$ | $-9 \leq L \leq 12$ | $-9 \leq L \leq 11$ |
| No. of ref. reflec. | 376 | 332 | 353 | 365 | 368 | 329 | 322 |
| No. of ref. param. | 15 | 15 | 15 | 15 | 15 | 15 | 15 |
| Data completeness | 22.8 | 21.7 | 21.7 | 21.1 | 21.3 | 20.8 | 19.7 |
| $U_{iso}$(Ir) | 0.0064(2) | 0.0124(3) | 0.0073(2) | 0.00623(18) | 0.0066(2) | 0.0044(3) | 0.0036(2) |
| $U_{iso}$(Li) | 0.0065(12) | 0.0132(18) | 0.0090(12) | 0.0056(10) | 0.0080(15) | 0.0119(19) | 0.0043(12) |
| $U_{iso}$(O) | 0.0065(12) | 0.0132(18) | 0.0090(12) | 0.0056(10) | 0.0080(15) | 0.0119(19) | 0.0043(12) |

TABLE S5. Structural parameters of $\beta$-$Li_2IrO_3$ at $P = 1.5$ GPa and $T = 50$ K. The space group is $P2_1/n$ (N° 14), $Z = 16$ and the lattice constants are $a = 5.8418(13)$ Å, $b = 16.445(1)$ Å, $c = 9.252(2)$ Å, $\beta = 107.62(2)°$ and $V = 847.2(3)$ Å$^3$. Site occupancy is 1 for all atoms; $U_{\text{iso}}$ is the isotropic displacement parameter and is given in Å$^2$ units. The final R factor is $R = 4.9\%$ and goodness of the fit $\chi^2 = 3.34$. No. of refined reflections: 1121; No. of fitted parameters: 51; Criterion for observed reflections: $I > 3\sigma(I)$.

| Atom | $x$ | $y$ | $z$ | $U_{iso}$ |
|---|---|---|---|---|
| Ir1 | 0.07461(19) | 0.18731(3) | 0.41245(16) | |
| Ir2 | 0.5932(2) | 0.43345(3) | 0.42158(17) | 0.00280(9) |
| Ir3 | 0.4139(2) | 0.43621(3) | 0.08167(17) | |
| Ir4 | 0.1052(2) | 0.68201(3) | 0.42746(17) | |
| Li1 | 0.2474(17) | 0.0594(2) | 0.2505(14) | |
| Li2 | 0.7382(17) | 0.3093(2) | 0.2438(14) | |
| Li3 | 0.9148(17) | 0.4356(2) | 0.0821(14) | |
| Li4 | 0.2374(17) | 0.3098(2) | 0.2440(14) | 0.0042(6) |
| Li5 | 0.4048(17) | 0.1866(2) | 0.0779(14) | |
| Li6 | 0.5694(17) | 0.1870(2) | 0.4106(14) | |
| Li7 | 0.2518(17) | 0.5595(2) | 0.2497(14) | |
| Li8 | 0.0835(17) | 0.4372(2) | 0.4160(14) | |
| O1 | 0.056(4) | 0.3083(5) | 0.409(3) | |
| O2 | 0.565(4) | 0.0575(5) | 0.416(3) | |
| O3 | 0.084(4) | 0.8022(5) | 0.424(3) | |
| O4 | 0.396(5) | 0.3154(5) | 0.072(4) | |
| O5 | 0.085(5) | 0.0652(5) | 0.422(4) | |
| O6 | 0.571(5) | 0.3117(5) | 0.412(4) | 0.0042(6) |
| O7 | 0.080(5) | 0.5601(5) | 0.415(4) | |
| O8 | 0.727(4) | 0.4337(5) | 0.245(3) | |
| O9 | 0.205(4) | 0.1856(5) | 0.239(3) | |
| O10 | 0.237(4) | 0.6845(5) | 0.252(3) | |
| O11 | 0.281(4) | 0.4353(5) | 0.256(3) | |
| O12 | 0.437(4) | 0.0541(5) | 0.086(3) | |

TABLE S6. Structural parameters of $\beta$-$Li_2IrO_3$ at $P = 2.0$ GPa and $T = 50$ K. The space group is $P2_1/n$ (N° 14), $Z = 16$ and the lattice constants are $a = 5.8383(7)$ Å, $b = 16.4217(5)$ Å, $c = 9.2429(11)$ Å, $\beta = 107.593(13)°$ and $V = 844.72(14)$ Å$^3$. Site occupancy is 1 for all atoms; $U_{\rm iso}$ is the isotropic displacement parameters and is given in Å$^2$ units. The final R factor is $R = 5.2\%$ and goodness of the fit $\chi^2 = 3.48$. No. of refined reflections: 1139; No. of fitted parameters: 51; Criterion for observed reflections: $I > 3\sigma(I)$.

| Atom | $x$ | $y$ | $z$ | $U_{iso}$ |
|---|---|---|---|---|
| Ir1 | 0.0753(2) | 0.18715(3) | 0.41272(16) | 0.00326(11) |
| Ir2 | 0.5927(3) | 0.43360(3) | 0.42143(17) | |
| Ir3 | 0.4144(3) | 0.43621(3) | 0.08174(17) | |
| Ir4 | 0.1048(2) | 0.68216(3) | 0.42729(16) | |
| Li1 | 0.2459(18) | 0.0591(2) | 0.2504(14) | 0.0052(7) |
| Li2 | 0.7412(17) | 0.3093(2) | 0.2442(14) | |
| Li3 | 0.9147(19) | 0.4354(2) | 0.0821(15) | |
| Li4 | 0.2379(17) | 0.3098(2) | 0.2442(14) | |
| Li5 | 0.4068(18) | 0.1863(2) | 0.0781(14) | |
| Li6 | 0.5698(17) | 0.1867(2) | 0.4106(14) | |
| Li7 | 0.2508(19) | 0.5593(2) | 0.2496(15) | |
| Li8 | 0.0850(19) | 0.4368(2) | 0.4163(15) | |
| O1 | 0.073(4) | 0.3086(7) | 0.416(3) | 0.0052(7) |
| O2 | 0.424(4) | 0.5579(7) | 0.078(3) | |
| O3 | 0.096(4) | 0.8036(7) | 0.430(3) | |
| O4 | 0.399(5) | 0.3152(7) | 0.073(4) | |
| O5 | 0.087(5) | 0.0649(7) | 0.421(4) | |
| O6 | 0.573(5) | 0.3119(7) | 0.412(4) | |
| O7 | 0.085(5) | 0.5602(7) | 0.414(4) | |
| O8 | 0.744(5) | 0.4323(5) | 0.251(4) | |
| O9 | 0.213(5) | 0.1850(5) | 0.244(4) | |
| O10 | 0.246(5) | 0.6839(5) | 0.257(4) | |
| O11 | 0.265(5) | 0.4344(5) | 0.250(4) | |
| O12 | 0.428(4) | 0.0545(7) | 0.081(3) | |

## REFERENCES

* l.veiga@ucl.ac.uk

† haskel@aps.anl.gov

[1] K. Momma and F. Izumi, Journal of Applied Crystallography **41**, 653 (2008).
